# Supplementary material for: On the Importance of Sampling in Training GCNs: Tighter Analysis and Variance Reduction
Source: arXiv:2103.02696 source file (2021-11-01)
Supplement: Supplementary file 1 [file proof_of_thm_1.tex]

\clearpage
\section{Proof of Theorem~\ref{theorem:convergence_of_sgcn}}
For the notation brevity, we first consider a special case of \texttt{SGCN}, a one layer GCN model, which is general enough to illustrate the main difficulties for sampling-based GCN training problems, but is also relatively simple so that we can clearly explain the main ideas and techniques required to handle these difficulties.
\begin{equation}
    \mathcal{L}(\bm{\theta}) = \frac{1}{N} \sum_{i=1}^N \text{Loss}\Big( \underbrace{\sum_{j=1}^N L_{i,j} \bm{x}_j \mathbf{W}^{(1)}}_{\bm{z}_i^{(1)}}, y_i \Big),~
    \widetilde{\mathcal{L}}(\bm{\theta}) = \frac{1}{B} \sum_{i\in\mathcal{V}_\mathcal{B}}\text{Loss} \Big( \underbrace{\sum_{j=1}^N \widetilde{L}^{(1)}_{i,j} \bm{x}_j \mathbf{W}^{(1)}}_{\widetilde{\bm{z}}_i^{(1)}}, y_i \Big)
\end{equation}
The gradient is calculated as 
\begin{equation}
    \nabla \mathcal{L}(\bm{\theta}) = \frac{1}{N} \sum_{i=1}^N \frac{\partial \text{Loss} ( \bm{z}_i^{(1)}, y_i)}{\partial \bm{z}_i^{(1)}} \Big( \sum_{j=1}^N L_{i,j} \bm{x}_j \Big),~
    \nabla \widetilde{\mathcal{L}}(\bm{\theta}) = \frac{1}{B} \sum_{i\in\mathcal{V}_\mathcal{B}} \frac{\partial \text{Loss} ( \widetilde{\bm{z}}_i^{(1)}, y_i)}{\partial \widetilde{\bm{z}}_i^{(1)}} \Big( \sum_{j=1}^N \widetilde{L}^{(1)}_{i,j} \bm{x}_j \Big)
\end{equation}

By bias-variance decomposition, we can decompose the mean-square error of stochastic gradient as
\begin{equation}
    \mathbb{E}[\|\nabla \widetilde{\mathcal{L}}(\bm{\theta}) - \nabla \mathcal{L}(\bm{\theta})\|_{\mathrm{F}}] = \underbrace{\mathbb{E}[\|\nabla \widetilde{\mathcal{L}}(\bm{\theta}) - \mathbb{E}[\nabla \mathcal{L}(\bm{\theta})] \|_{\mathrm{F}}]}_{variance}  + \underbrace{\mathbb{E}[\|\mathbb{E}[\nabla \mathcal{L}(\bm{\theta})]  - \nabla \mathcal{L}(\bm{\theta})\|_{\mathrm{F}}] }_{bias}
\end{equation}
where $\mathbb{E}[\nabla \mathcal{L}(\bm{\theta})] $ is computed as
\begin{equation}
    \mathbb{E}[\nabla \mathcal{L}(\bm{\theta})] = \frac{1}{N} \sum_{i=1}^N \frac{\partial \text{Loss} ( \widetilde{\bm{z}}_i^{(1)}, y_i)}{\partial \widetilde{\bm{z}}_i^{(1)}} \Big( \sum_{j=1}^N L_{i,j} \bm{x}_j \Big)
\end{equation}

Therefore, we can bound the variance term as
\begin{equation}
    \begin{aligned}
    &\mathbb{E}[\|\nabla \widetilde{\mathcal{L}}(\bm{\theta}) - \mathbb{E}[\nabla \mathcal{L}(\bm{\theta})] \|_{\mathrm{F}}] \\
    &= \mathbb{E}\Big[ \Big\| \frac{1}{B} \sum_{i\in\mathcal{V}_\mathcal{B}} \frac{\partial \text{Loss} ( \widetilde{\bm{z}}_i^{(1)}, y_i)}{\partial \widetilde{\bm{z}}_i^{(1)}} \Big( \sum_{j=1}^N \widetilde{L}^{(1)}_{i,j} \bm{x}_j \Big) - \frac{1}{N} \sum_{i=1}^N \frac{\partial \text{Loss} ( \widetilde{\bm{z}}_i^{(1)}, y_i)}{\partial \widetilde{\bm{z}}_i^{(1)}} \Big( \sum_{j=1}^N L_{i,j} \bm{x}_j \Big) \Big\|_{\mathrm{F}} \Big] \\
    &\leq \mathbb{E}\Big[ \Big\| \frac{1}{B} \sum_{i\in\mathcal{V}_\mathcal{B}} \frac{\partial \text{Loss} ( \widetilde{\bm{z}}_i^{(1)}, y_i)}{\partial \widetilde{\bm{z}}_i^{(1)}} \Big( \sum_{j=1}^N \widetilde{L}^{(1)}_{i,j} \bm{x}_j \Big) - \frac{1}{B} \sum_{i\in\mathcal{V}_\mathcal{B}} \frac{\partial \text{Loss} ( \widetilde{\bm{z}}_i^{(1)}, y_i)}{\partial \widetilde{\bm{z}}_i^{(1)}} \Big( \sum_{j=1}^N L_{i,j} \bm{x}_j \Big) \Big\|_{\mathrm{F}} \Big] \\
    &\quad + \mathbb{E}\Big[ \Big\| \frac{1}{B} \sum_{i\in\mathcal{V}_\mathcal{B}} \frac{\partial \text{Loss} ( \widetilde{\bm{z}}_i^{(1)}, y_i)}{\partial \widetilde{\bm{z}}_i^{(1)}} \Big( \sum_{j=1}^N L_{i,j} \bm{x}_j \Big) - \frac{1}{N} \sum_{i=1}^N \frac{\partial \text{Loss} ( \widetilde{\bm{z}}_i^{(1)}, y_i)}{\partial \widetilde{\bm{z}}_i^{(1)}} \Big( \sum_{j=1}^N L_{i,j} \bm{x}_j \Big) \Big\|_{\mathrm{F}} \Big]
    \end{aligned}
\end{equation}

We can bound the variance term as
\begin{equation}
    \begin{aligned}
    &\mathbb{E}[\|\mathbb{E}[\nabla \mathcal{L}(\bm{\theta})]  - \nabla \mathcal{L}(\bm{\theta})\|_{\mathrm{F}}] \\
    &= \mathbb{E}\Big[ \Big\| \frac{1}{N} \sum_{i=1}^N \frac{\partial \text{Loss} ( \widetilde{\bm{z}}_i^{(1)}, y_i)}{\partial \widetilde{\bm{z}}_i^{(1)}} \Big( \sum_{j=1}^N L_{i,j} \bm{x}_j \Big) - \frac{1}{N} \sum_{i=1}^N \frac{\partial \text{Loss} ( \bm{z}_i^{(1)}, y_i)}{\partial \bm{z}_i^{(1)}} \Big( \sum_{j=1}^N L_{i,j} \bm{x}_j \Big) \Big\|_{\mathrm{F}} \Big] \\
    &=\mathbb{E}\Big[ \Big\| \frac{1}{N} \sum_{i=1}^N \Big( \frac{\partial \text{Loss} ( \widetilde{\bm{z}}_i^{(1)}, y_i)}{\partial \widetilde{\bm{z}}_i^{(1)}} - \frac{\partial \text{Loss} ( \bm{z}_i^{(1)}, y_i)}{\partial \bm{z}_i^{(1)}} \Big) \Big( \sum_{j=1}^N L_{i,j} \bm{x}_j \Big) \Big\|_{\mathrm{F}} \Big] 
    \end{aligned}
\end{equation}

\textcolor{red}{======================}

\begin{equation}
    \mathbf{D}^{(L+1)} = \frac{\partial \mathcal{L}(\bm{\theta)}}{\partial \mathbf{H}^{(1)}} \in\mathbb{R}^{1 \times N \times d_1},~
    \widetilde{\mathbf{D}}^{(L+1)} = \frac{\partial \widetilde{\mathcal{L}}(\bm{\theta)}}{\partial \widetilde{\mathbf{H}}^{(L)}} \in\mathbb{R}^{1 \times N \times d_1}
\end{equation}

\begin{equation}
    \mathbf{G}^{(1)} = \frac{\partial \sigma(\mathbf{L} \mathbf{X} \mathbf{W}^{(1)} )}{\partial \mathbf{W}^{(1)} } \in \mathbb{R}^{N \times d_1 \times d_0},
    \widetilde{\mathbf{G}}^{(\ell)} = \frac{\partial \sigma(\widetilde{\mathbf{L}}^{1)} \mathbf{X} \mathbf{W}^{(1)} )}{\partial \mathbf{W}^{(1)} } \in \mathbb{R}^{N \times d_1 \times d_0 }
\end{equation}
