# Supplementary material for: On the Importance of Sampling in Training GCNs: Tighter Analysis and Variance Reduction
Source: arXiv:2103.02696 source file (2021-11-01)
Supplement: Supplementary file 2 [file reproduce.tex]

\section{Reproducing experiment results}
To reproduce the results reported in the paper, we provide link for dataset download, the bash script to reproduce the experiment results, and a jupyter notebook file for a quick visualization and GPU utilization calculation. It is worth noting that due to the existence of randomness, the obtained results (e.g., loss curve) may be slightly different. However, it is not difficult to find that the overall trend of loss curves and conclusions will remains the same.

This implementation is based on \footnote{\url{https://pytorch.org/}}{PyTorch} using Python 3. We notice that Python 2 might results in a wrong gradient update, even for vanilla \texttt{SGCN}s. 

Install dependencies:
% \begin{minted}{bash}
\begin{minted}[fontsize=\small]{bash}
    # create virtual environment
    $ virtualenv env
    $ source env/bin/activate
    # install dependencies 
    $ pip install -r requirements.txt
\end{minted}

Experiments are produced on PPI, PPI-Large, Flickr, Reddit, and Yelp datasets. 
The utilized datasets can be downloaded from the Google drive folder\footnote{\url{https://drive.google.com/drive/folders/15eP7OHiHQUnDrHKYh1YPxXkiqGoJhbis?usp=sharing}}.
% \begin{minted}{bash}
\begin{minted}[fontsize=\small, tabsize=2,breaklines]{bash}
    # create folders that save experiment results and datasets
    $ mkdir ./results
    $ mkdir ./data # please download the dataset and put them inside this folder
\end{minted}

To reproduce the results, please run the following commands:
% \begin{minted}{bash} % change for arxiv version
\begin{minted}[fontsize=\small]{bash}
    $ python train.py --sample_method 'ladies' --dataset 'reddit' 
    $ python train.py --sample_method 'fastgcn' --dataset 'reddit' 
    $ python train.py --sample_method 'graphsage' --dataset 'reddit' 
    $ python train.py --sample_method 'vrgcn' --dataset 'reddit' 
    $ python train.py --sample_method 'graphsaint' --dataset 'reddit' 
    $ python train.py --sample_method 'exact' --dataset 'reddit' 
    
    $ python train.py --sample_method 'ladies' --dataset 'ppi'
    $ python train.py --sample_method 'fastgcn' --dataset 'ppi'
    $ python train.py --sample_method 'graphsage' --dataset 'ppi'
    $ python train.py --sample_method 'vrgcn' --dataset 'ppi'
    $ python train.py --sample_method 'graphsaint' --dataset 'ppi'
    $ python train.py --sample_method 'exact' --dataset 'ppi'
    
    $ python train.py --sample_method 'ladies' --dataset 'flickr'
    $ python train.py --sample_method 'fastgcn' --dataset 'flickr'
    $ python train.py --sample_method 'graphsage' --dataset 'flickr'
    $ python train.py --sample_method 'vrgcn' --dataset 'flickr'
    $ python train.py --sample_method 'graphsaint' --dataset 'flickr'
    $ python train.py --sample_method 'exact' --dataset 'flickr'
    
    $ python train.py --sample_method 'ladies' --dataset 'ppi-large'
    $ python train.py --sample_method 'fastgcn' --dataset 'ppi-large'
    $ python train.py --sample_method 'graphsage' --dataset 'ppi-large'
    $ python train.py --sample_method 'vrgcn' --dataset 'ppi-large'
    $ python train.py --sample_method 'graphsaint' --dataset 'ppi-large'
    $ python train.py --sample_method 'exact' --dataset 'ppi-large'
    
    $ python train.py --sample_method 'ladies' --dataset 'yelp'
    $ python train.py --sample_method 'fastgcn' --dataset 'yelp'
    $ python train.py --sample_method 'graphsage' --dataset 'yelp'
    $ python train.py --sample_method 'vrgcn' --dataset 'yelp'
    $ python train.py --sample_method 'graphsaint' --dataset 'yelp'
    $ python train.py --sample_method 'exact' --dataset 'yelp'   
\end{minted}
