# Supplementary material for: On the Importance of Sampling in Training GCNs: Tighter Analysis and Variance Reduction
Source: arXiv:2103.02696 source file (2021-11-01)
Supplement: Supplementary file 3 [file sampling_algorithms.tex]

% \section{Different sampling strategies}\label{supp:diff_sampling_strategy}
% \mr{move to main}

% In this section, we highlight the difference between node-wise sampling, layer-wise sampling, and subgraph sampling algorithms.

% \paragraph{Node-wide sampling.}~
% The main idea of node-wise sampling is to first sample all the nodes needed for the computation using neighbor sampling (NS), then train the GCN based on the sampled nodes. 
% For each node in the $\ell$th GCN layer, NS randomly samples $s$ of its neighbors at the $(\ell-1)$th GCN layer and formulate $\widetilde{\mathbf{L}}^{(\ell)}$ by
% \begin{equation}\label{eq:node_wise}
%     \widetilde{L}_{i,j}^{(\ell)} = \begin{cases}
%  \frac{|\mathcal{N}(i)|}{s} \times {L}_{i,j}, &\text{ if } j \in \widetilde{\mathcal{N}}^{(\ell)}(i) \\
%  0, &\text{ otherwise }
% \end{cases}
% \end{equation}
% where $\mathcal{N}(i)$ is the full set of $i$th node neighbor, $\widetilde{\mathcal{N}}^{(\ell)}(i)$ is the sampled neighbors of node $i$ for $\ell$th GCN layer.
% \texttt{GraphSAGE}~\cite{graphsage} follows the spirit of node-wise sampling where it performs uniform node sampling on the previous layer neighbors for a fixed number of nodes to bound the mini-batch computation complexity. 

% \paragraph{Layer-wise sampling.}~
% To avoid the neighbor explosion issue, layer-wise sampling is introduced to controls the size of sampled neighborhoods in each layer. 
% For the $\ell$th GCN layer, layer-wise sampling methods sample a set of nodes $\mathcal{B}^{(\ell)}\subseteq\mathcal{V}$ of size $s$ under the distribution $\boldsymbol{p}$ to approximate the Laplacian by
% \begin{equation}\label{eq:layer-wise}
%     \widetilde{L}_{i,j}^{(\ell)} = \begin{cases}
%  \frac{1}{s \times p_j}\times {L}_{i,j}, &\text{ if } j \in \mathcal{B}^{(\ell)} \\
%  0, &\text{ otherwise }
% \end{cases}
% \end{equation}

% Existing work \texttt{FastGCN}~\cite{fastgcn} and \texttt{LADIES}~\cite{ladies} follows the spirit of layer-wise sampling.
% \texttt{FastGCN} performs independently node sampling for each layer and applies important sampling to reduce variance and results in a constant sample size in all layers. 
% However, mini-batches potentially become too sparse to achieve high accuracy. 
% \texttt{LADIES} improves \texttt{FastGCN} by layer-dependent sampling. 
% Based on the sampled nodes in the upper layer, it selects their neighborhood nodes, constructs a bipartite subgraph, and computes the importance probability accordingly. 
% Then, it samples a fixed number of nodes based on the calculated probability, and recursively conducts such a procedure per layer to construct the whole computation graph. 

% \paragraph{Subgraph sampling.}~ 
% Subgraph sampling is similar to layer-wise sampling by restricting the sampled Laplacian matrices at each layer are identical
% \begin{equation}\label{eq:graph-wise}
%     \widetilde{L}_{i,j}^{(1)} = \ldots = \widetilde{L}_{i,j}^{(L)} = \begin{cases}
%  \frac{1}{s \times p_j}\times {L}_{i,j}, &\text{ if } j \in \mathcal{B}^{(\ell)} \\
%  0, &\text{ otherwise }
% \end{cases}
% \end{equation}
% For example, \texttt{GraphSAINT}~\cite{graphsaint} can be viewed as a special case of layer-wise sampling algorithm \texttt{FastGCN} by restricting the nodes sampled at the $1$-st to $(L-1)$th layer the same as the nodes sampled at the $L$th layer. 
% However, \texttt{GraphSAINT} requires a significant large mini-batch size compared to other layer-wise sampling methods. 
% We leave this as a potential future direction to explore.
