# Supplementary material for: On the Importance of Sampling in Training GCNs: Tighter Analysis and Variance Reduction
Source: arXiv:2103.02696 source file (2021-11-01)
Supplement: Supplementary file 4 [file additional_experiments.tex]

% \clearpage
% \section{Additional experiments}~\label{section:additional_exps}

% \noindent\textbf{Effect of variance reduction.}~
% In Figure~\ref{fig:mse_compare}, we empirically evaluate the effectiveness of variance reduction by comparing the mean-square error of the stochastic gradient and training loss curve of different sampling strategies on \texttt{Reddit} dataset. 

% Because \texttt{Exact} sampling is using all neighbors for the node embedding approximation, it is only affected by layerwise gradient variance (first-order variance). 
% Therefore, employing first-order variance reduction on \texttt{Exact} sampling can significantly reduce the mean-square error of stochastic gradient to full-gradient, and speed up the convergence. 

% Different from \texttt{Exact} sampling that the exact node embeddings are available during training, layerwise sampling algorithm \texttt{LADIES}, and nodewise sampling \texttt{GraphSAGE} are approximating the true node embeddings using a subset of nodes (neighbors).
% Therefore, these methods both suffer from node embedding approximation variance (zeroth-order variance) and layerwise gradient variance (first-order variance).  As a result, applying zeroth-order variance reduction and first-order variance reduction simultaneously is necessary to reduce the mean-square error of the stochastic gradient and speed up the convergence.
% \begin{figure}[h]
%     \centering
%     \includegraphics[width=1.0\textwidth]{experiment_figures/mse_compare/mse_compare.pdf}
%     \caption{Comparing the mean-square error of stochastic gradient to full gradient and training loss of \texttt{SGCN}, \texttt{SGCN+}, \texttt{SGCN++} in the first $200$ iterations of training process on \texttt{Reddit} dataset.}
%     \label{fig:mse_compare}
% \end{figure}

% \textcolor{red}{
% \noindent\textbf{Extension to bandit sampling.}
% Most recently, \cite{liu2020bandit,zhang2021biased} propose bandit sampling strategy to approximate the importance sampling distribution using multi-armed bandit. The key idea is to assign each neighbor an importance sampling weight $w_j, j\in\mathcal{N}(i)$, then used the gradient of the embedding approximation variance of sampling node $j$ as the neighbor of node $i$ as a feedback to update weight $w_j$. 
% When using zeroth order variance reduction (\texttt{Bandit+}) and first order variance reduction (\texttt{Bandit++}) with bandit sampling, one of the biggest benefit is that we can directly used the historical node embeddings to approximate the importance sampling distribution, without worrying about the instability of the bandit feedback as mentioned by \cite{zhang2021biased}.
% In the following, we compare the convergence of \texttt{Bandit+} and \texttt{Bandit++}
% }


% \clearpage
% \noindent\textbf{GPU memory usage.}~
% In Figure~\ref{fig:gpu_utils}, We compare the GPU memory usage of \texttt{SGCN} and \texttt{SGCN++}.
% We calculate the allocated memory by \texttt{torch.cuda.memory\_allocated}, which is the current GPU memory occupied by tensors in bytes for a given device. 
% We calculate the maximum allocated memory by \texttt{torch.cuda.max\_memory\_allocated}, which is the maximum GPU memory occupied by tensors in bytes for a given device.

% From Figure~\ref{fig:gpu_utils}, we observe that neither running full-batch GCN nor saving historical node embeddings and gradients will significantly increase the computation overhead during training.
% Besides, since all historical activations are stored outside GPU, we see that \texttt{SGCN++} only requires several megabytes to transfer data between GPU memory to the host, which can be ignored compared to the memory usage of calculation itself. 
% % As a result, we can conclude that the bottleneck of training sampling-based GCNs is sampling rather than computation. 
% % Therefore, a promising future direction is developing a provable sampling algorithm with low sampling complexity.

% \begin{figure}[h]
%     \centering
%     \includegraphics[width=0.7\textwidth]{experiment_figures/gpu_utils.pdf}
%     \caption{Comparison of GPU memory usage of \texttt{SGCN} and \texttt{SGCN++} on Flickr and PPI dataset.}
%     \label{fig:gpu_utils}
% \end{figure}

% % \clearpage
% \begin{figure}
%     \centering
%     \includegraphics[width=1.0\textwidth]{figures/reddit-wall-clock.pdf}
%     \caption{Comparison of training and validation loss of \texttt{SGCN}, \texttt{SGCN+}, \texttt{SGCN++} using wall clock time on \texttt{Reddit} dataset. }
%     \label{fig:reddit-wall-clock}
% \end{figure}

% \begin{figure}
%     \centering
%     \includegraphics[width=1.0\textwidth]{figures/ppi-large-wall-clock.pdf}
%     \caption{Comparison of training and validation loss of \texttt{SGCN}, \texttt{SGCN+}, \texttt{SGCN++} using wall clock time on \texttt{PPI-Large} dataset. }
%     \label{fig:ppi-large-wall-clock}
% \end{figure}
% \noindent\textbf{Evaluation of total time}.~
% In Table~\ref{table:doubly_ladies_time} and Table~\ref{table:ladies_time}, we report the average time of doubly variance reduced \texttt{LADIES++} and vanilla \texttt{LADIES}. We classify the wall clock time during the training process into five categories:
% \begin{itemize}
%     \item \textbf{Snapshot step sampling time}: The time used to construct the snapshot full-batch or the snapshot large-batch. In practice, we directly use full-batch training for the smaller datasets (e.g., PPI, PPI-large, and Flickr) and use sampled snapshot large-batch for large datasets (e.g., Reddit and Yelp). When constructing snapshot large-batch, the \texttt{Exact} sampler has to go through all neighbors of each node using for-loops based on the graph structure, such that it is time-consuming.
%     \item \textbf{Snapshot step transfer time}: The time required to transfer the sampled snapshot batch nodes and Laplacian matrices to the GPUs.
%     \item \textbf{Regular step sampling time}: The time used to construct the mini-batches using layerwise \texttt{LADIES} sampler. 
%     \item \textbf{Regular step transfer time}: The time required to transfer the sampled mini-batch nodes and Laplacian matrices to GPUs, and the time to transfer the historical node embeddings and the stochastic gradient between GPUs and CPUs.
%     \item \textbf{Computation time}: The time used for forward- and backward-propagation.
% \end{itemize}

% Notice that we are reporting the total time per iteration because the vanilla sampling-based method cannot reach the same accuracy as the doubly variance reduced algorithm (due to the residual error as shown in Theorem~\ref{theorem:convergence_of_sgcn}).

% From Table~\ref{table:doubly_ladies_time} and Table~\ref{table:ladies_time}, we can observe that the most time-consuming process in sampling-based GCN training is data sampling and data transfer.
% The extra computation time introduces by employing the snapshot step is negligible when comparing to the mini-batch sampling time during each regular step.
% % Since doubly variance reduction can give us a better convergence and generalization performance, t
% Therefore, a promising future direction for large-scale graph training is developing a provable sampling algorithm with low sampling complexity.
% Besides, in Figure~\ref{fig:reddit-wall-clock} and Figure~\ref{fig:ppi-large-wall-clock}, we compare the wall clock time of all methods on \texttt{PPI-large} and \texttt{Reddit dataset} with the default setup as introduced in Section~\ref{section:exp-config}. From Figure~\ref{fig:reddit-wall-clock} and Figure~\ref{fig:ppi-large-wall-clock}, we can observe that although \texttt{SGCN+} and \texttt{SGCN++} sometime require more wall-clock time, they can get a better training and validation result than vanilla \texttt{SGCN}.

% \input{supplementary/table_time_summary}

% % \clearpage
% \noindent\textbf{Evaluation of snapshot gap for \texttt{SGCN+} and \texttt{SGCN++}.}~
% Doubly variance reduced \texttt{SGCN++} requires performing full-batch (large-batch) training periodically to calculate the snapshot node embeddings and gradients. 
% A larger snapshot gap $K$ can make training faster, but also might make the snapshot node embeddings and gradients too stale for variance reduction. 
% In this experiment, we evaluate the effect of snapshot grap on training by choosing mini-batch size as $B=512$, disable the early stop criterion, and change the inner-loop intervals from $K=5$ mini-batches to $K=20$ mini-batches.
% In Figure~\ref{fig:change_of_K} and Figure~\ref{fig:change_k_zeroth_result}, we show the comparison of training loss and validation loss with different number of inner-loop intervals for \texttt{SGCN++} and \texttt{SGCN+} on \texttt{Reddit} dataset, respectively.
% We can observe that the model with a smaller snapshot gap requires less number of iterations to reach the same training and validation loss, and gives us a better generalization performance (F1-score).


% \begin{figure}[h]
%     \centering
%     \includegraphics[width=1\textwidth]{experiment_figures/change_of_K.pdf}
%     \caption{Comparison of training loss, validation loss, and F1-score of \texttt{SGCN++} with different snapshot gap on \texttt{Reddit} dataset. }
%     \label{fig:change_of_K}
% \end{figure}

% \begin{figure}
%     \centering
%     \includegraphics[width=1\textwidth]{figures/change_k_zeroth_result.pdf}
%     \caption{Comparison of training loss, validation loss, and F1-score of \texttt{SGCN+} with different snapshot gap on \texttt{Reddit} dataset.}
%     \label{fig:change_k_zeroth_result}
% \end{figure}

% % \clearpage
% {\noindent\textbf{Evaluation of large-batch size for \texttt{SGCN+} and \texttt{SGCN++}}.~
% The full-batch gradient calculation at each snapshot step is computationally expensive. 
% Heuristically, we can approximate the full-batch gradient by using the gradient computed on a large-batch of nodes. 
% Besides, it is worth noting that large-batch approximation can be also used for the node embedding approximation in zeroth-order variance reduction. 
% In \texttt{SGCN+}, saving the historical node embeddings for all nodes in an extreme large graph can be computationally prohibitive. 
% An alternative strategy is sampling a large-batch during the snapshot step, computing the node embeddings for all nodes in the large-batch, and saving the freshly computed node embeddings on the storage. After that, mini-batch nodes are sampled from the large-batch during the regular steps.
% Let denote $B^\prime$ as the snapshot step large-batch size and $B$ denote the regular step mini-batch size. 
% By default, we choose snapshot gap as $K=10$, disable the early stop criterion, fix the regular step batch size as $B=512$, and change the snapshot step batch size $B^\prime$ from $20,000$ (20K) to $80,000$ (80K).
% In Figure~\ref{fig:chang_B_prime} and Figure~\ref{fig:change_K_zeroth}, we show the comparison of training loss and validation loss with different snapshot step large-batch size $B^\prime$ for \texttt{SGCN++} and \texttt{SGCN+}, respectively. 
% }

% \begin{figure}[h]
%     \centering
%     \includegraphics[width=1.0\textwidth]{experiment_figures/chang_B_prime.pdf}
%     \caption{{Comparison of training loss, validation loss, and F1-score of \texttt{SGCN++} with different snapshot large-batch size on \texttt{Reddit} dataset.}}
%     \label{fig:chang_B_prime}
% \end{figure}


% \begin{figure}
%     \centering
%     \includegraphics[width=1.0\textwidth]{figures/change_K_zeroth.pdf}
%     \caption{{Comparison of training loss, validation loss, and F1-score of \texttt{SGCN+} with different snapshot large-batch size on \texttt{Reddit} dataset.}}
%     \label{fig:change_K_zeroth}
% \end{figure}

% % \clearpage
% % \noindent\textbf{The effect of mini-batch size.}~
% % In Figure~\ref{fig:change_mini_batch}, we show the comparsion of training loss and validation loss with different regular step mini-batch size. 
% % By default, we choose the snapshot gap as $K=10$ , fix the snapshot step batch size as $B^\prime = 80,000$, and change the regular step mini-batch size $B$ from $256$ to $2,048$.
% % Besides, we note that subgraph sampling algorithm \texttt{GraphSAINT} requires an extreme large mini-batch size every iterations. In Figure~\ref{fig:graphsaint_batch_size}, we explicitly compare the effectiveness of mini-batch size on doubly variance reduced \texttt{GraphSAINT++} and vanilla \texttt{GraphSAINT}, and show that a smaller mini-batch is required by \texttt{GraphSAINT++}.

% % \begin{figure}[h]
% %     \centering
% %     \includegraphics[width=1.0\textwidth]{experiment_figures/batch_size/change_mini_batch.pdf}
% %     \caption{Comparison of training loss, validation loss, and F1-score of \texttt{SGCN++} with different mini-batch size on \texttt{Reddit} dataset.}
% %     \label{fig:change_mini_batch}
% % \end{figure}

% % \begin{figure}[h]
% %     \centering
% %     \includegraphics[width=0.35\textwidth]{experiment_figures/batch_size/addition_exps_val.pdf}
% %     \caption{Comparing the validation loss and F1-score of \texttt{GraphSAINT} and \texttt{GraphSAINT++} with different mini-batch size on \texttt{Reddit} dataset}
% %     \label{fig:graphsaint_batch_size}
% % \end{figure}

% {
% \noindent\textbf{Evaluation of increasing snapshot gap.}
% Snapshot gap size $K$ serves as a budge hyper-parameter that balances between training speed and the quality of variance reduction. 
% During training, as the number of iterations increases, the GCN models convergences to a saddle point. Therefore, it is interesting to explore whether increasing the snapshot gap $K$ during the training process can obtain a speed boost. In Figure~\ref{fig:change_K_valid_loss}, we show the comparison of validation loss of fixed snapshot gap $K=10$ and gradually increasing snapshot gap $K=10+0.1\times s, s=1,2,\ldots$, where $s$ is the number of snapshot steps has been computed. 
% We disable the early stop criterion so that we can run the desired number of inner-loop steps without being affected by early stopping.
% Recall that the key bottleneck for \texttt{SGCN++} is memory budget and sampling complexity, rather than snapshot computing. Dynamically increasing snapshot gap can reduce the number of snapshot steps, but cannot significantly reduce the training time but might lead to a performance drop.
% }

% \begin{figure}
%     \centering
%     \includegraphics[width=1.0\textwidth]{figures/change_K_valid_loss.pdf}
%     \caption{{Effectiveness of gradually increasing snapshot gap $K$ during training on wallclock time (second) and accuracy on \texttt{PPI} dataset. We choose snapshot gap $K=10$ for fixed-$K$. For increasing $K$, we choose snapshot gap $K=10+0.1\times s, s=1,2,\ldots$, where $s$ is the number of snapshot steps.}}
%     \label{fig:change_K_valid_loss}
% \end{figure}

% \begin{figure}[h]
%     \centering
%     \includegraphics[width=1.0\textwidth]{experiment_figures/change_mini_batch.pdf}
%     \caption{Comparison of training loss, validation loss, and F1-score of \texttt{SGCN++} with different mini-batch size on \texttt{PPI-Large} dataset.}
%     \vspace{10pt}
%     \label{fig:change_mini_batch}
% \end{figure}

% \noindent\textbf{The effect of mini-batch size.}~
% In Figure~\ref{fig:change_mini_batch}, we show the comparsion of training loss and validation loss with different regular step mini-batch size. 
% By default, we choose the snapshot gap as $K=10$, fix the snapshot step batch size as $B^\prime = 80,000$, disable the early stop criterion, and change the regular step mini-batch size $B$ from $256$ to $2,048$.
% Besides, we note that subgraph sampling algorithm \texttt{GraphSAINT} requires an extreme large mini-batch size every iterations. In Figure~\ref{fig:graphsaint_batch_size}, we explicitly compare the effectiveness of mini-batch size on doubly variance reduced \texttt{GraphSAINT++} and vanilla \texttt{GraphSAINT}, and show that a smaller mini-batch is required by \texttt{GraphSAINT++}.


% \begin{figure}[h]
%     \centering
%     \includegraphics[width=0.5\textwidth]{experiment_figures/addition_exps_val.pdf}
%     \caption{Comparing the validation loss and F1-score of \texttt{GraphSAINT} and \texttt{GraphSAINT++} with different mini-batch size on \texttt{Reddit} dataset}
%     \label{fig:graphsaint_batch_size}
% \end{figure}
