# Supplementary material for: On the Importance of Sampling in Training GCNs: Tighter Analysis and Variance Reduction
Source: arXiv:2103.02696 source file (2021-11-01)
Supplement: Supplementary file 6 [file convergence_of_fullgcn.tex]

\section{Convergence of \texttt{FullGCN}}
Let first recall the parameters and gradients of a $L$-layer GCN is defined as
\begin{equation}
\bm{\theta} = \{ \mathbf{W}^{(1)}, \ldots, \mathbf{W}^{(L)} \},~
\nabla \mathcal{L}(\bm{\theta}) = \{\mathbf{G}^{(1)}, \ldots, \mathbf{G}^{(L)}\}
\end{equation}
where $\mathbf{G}^{(\ell)}$ is defined as the gradient w.r.t. the $\ell$th layer weight matrix. Let us slight abuse of notation and define the distance between two set of parameters $\bm{\theta}_1, \bm{\theta}_2$ and its gradient as
\begin{equation}
    \| \bm{\theta}_1-\bm{\theta}_2\|_{\mathrm{F}}^2 = \sum_{\ell=1}^L \| \mathbf{W}_1^{(\ell)} - \mathbf{W}_2^{(\ell)}\|_{\mathrm{F}}^2,~
    \| \nabla\mathcal{L}( \bm{\theta}_1)-\nabla \mathcal{L}(\bm{\theta}_2)\|_{\mathrm{F}}^2 = \sum_{\ell=1}^L \| \mathbf{G}_1^{(\ell)} - \mathbf{G}_2^{(\ell)}\|_{\mathrm{F}}^2
\end{equation}

We first derive the smoothness constant of a $L$-layer graph convolutonal network.
\begin{lemma} \label{lemma:smoothness_L_layer}
The gradient of an $L$-layer GCN is $L_f$-Lipschitz continuous with $L_f=L(2L+1)(L U_{\max L}^2 U_{\max C}^2 + U_{\max L}^2 )$, i.e.,
\begin{equation}
    \|\nabla \mathcal{L}(\bm{\theta}_1) - \nabla \mathcal{L}(\bm{\theta}_2)\|_{\mathrm{F}}^2 \leq L_f \| \bm{\theta}_1-\bm{\theta}_2\|_{\mathrm{F}}^2
\end{equation}

where
\begin{equation}
    \begin{aligned}
    U_C(a,b) &= \begin{cases}
        C_{Wa} \Big( \prod_{c=a+1}^b C_{Hc} \Big) & \text{ if } b \geq a+1 \\ 
        C_{Wa} & \text{ otherwise } 
    \end{cases} \\
    U_L(a,b) &= \begin{cases}
    L_{Wa} \Big( \prod_{c=a+1}^b L_{Hc} \Big) & \text{ if } b \geq a + 1 \\ 
    L_{Wa}  & \text{ otherwise } 
\end{cases} \\
    \end{aligned}
\end{equation}
and
\begin{equation}
\begin{aligned}
U_{\max C} &= \max_{a,b\in[L]} U_C(a,b) \\
U_{\max L} &= \max\Big\{\max_{a,b\in[L]} U_L(a,b), \max_{a,b\in[L]} U_L(a,b) \times L_\text{loss}\Big\}
\end{aligned}
\end{equation}

\end{lemma}
\begin{proof}

We first consider the gradient w.r.t. the $\ell$th graph convolutional layer weight matrix
\begin{equation}
    \begin{aligned}
    &\| \mathbf{G}_1^{(\ell)} - \mathbf{G}_2^{(\ell)}\|_{\mathrm{F}}^2 \\
    &= \|\nabla_W f^{(\ell)}( \nabla_H f^{(\ell+1)}( \ldots \nabla_H f^{(L)}( \mathbf{D}^{(L+1)}_1, \mathbf{H}_1^{(L-1)}, \mathbf{W}_1^{(L)}) \ldots, \mathbf{H}_1^{(\ell)}, \mathbf{W}_1^{(\ell+1)}) , \mathbf{H}_1^{(\ell-1)}, \mathbf{W}_1^{(\ell)}) \\
    &\quad - \nabla_W f^{(\ell)}( \nabla_H f^{(\ell+1)}( \ldots \nabla_H f^{(L)}( \mathbf{D}^{(L+1)}_2, \mathbf{H}_2^{(L-1)}, \mathbf{W}_2^{(L)}) \ldots,\mathbf{H}_2^{(\ell)} \mathbf{W}_2^{(\ell+1)}) , \mathbf{H}_2^{(\ell-1)}, \mathbf{W}_2^{(\ell)}) \|_{\mathrm{F}}^2 \\
    &\leq (2L+1) \times \Big( \| \nabla_W f^{(\ell)}( \nabla_H f^{(\ell+1)}( \ldots \nabla_H f^{(L)}( \mathbf{D}^{(L+1)}_1, \mathbf{H}_1^{(L-1)}, \mathbf{W}_1^{(L)}) \ldots, \mathbf{H}_1^{(\ell)}, \mathbf{W}_1^{(\ell+1)}) , \mathbf{H}_1^{(\ell-1)}, \mathbf{W}_1^{(\ell)}) \\
    &\quad - \nabla_W f^{(\ell)}( \nabla_H f^{(\ell+1)}( \ldots \nabla_H f^{(L)}( \mathbf{D}^{(L+1)}_2, \mathbf{H}_1^{(L-1)}, \mathbf{W}_1^{(L)}) \ldots, \mathbf{H}_1^{(\ell)}, \mathbf{W}_1^{(\ell+1)}) , \mathbf{H}_1^{(\ell-1)}, \mathbf{W}_1^{(\ell)}) \|_{\mathrm{F}}^2  \\
    &\quad + \| \nabla_W f^{(\ell)}( \nabla_H f^{(\ell+1)}( \ldots \nabla_H f^{(L)}( \mathbf{D}^{(L+1)}_2, \mathbf{H}_1^{(L-1)}, \mathbf{W}_1^{(L)}) \ldots, \mathbf{H}_1^{(\ell)}, \mathbf{W}_1^{(\ell+1)}) , \mathbf{H}_1^{(\ell-1)}, \mathbf{W}_1^{(\ell)}) \\
    &\quad - \nabla_W f^{(\ell)}( \nabla_H f^{(\ell+1)}( \ldots \nabla_H f^{(L)}( \mathbf{D}^{(L+1)}_2, \mathbf{H}_2^{(L-1)}, \mathbf{W}_1^{(L)}) \ldots, \mathbf{H}_1^{(\ell)}, \mathbf{W}_1^{(\ell+1)}) , \mathbf{H}_1^{(\ell-1)}, \mathbf{W}_1^{(\ell)}) \|_{\mathrm{F}}^2 \\ 
    &\quad + \| \nabla_W f^{(\ell)}( \nabla_H f^{(\ell+1)}( \ldots \nabla_H f^{(L)}( \mathbf{D}^{(L+1)}_2, \mathbf{H}_2^{(L-1)}, \mathbf{W}_1^{(L)}) \ldots, \mathbf{H}_1^{(\ell)}, \mathbf{W}_1^{(\ell+1)}) , \mathbf{H}_1^{(\ell-1)}, \mathbf{W}_1^{(\ell)}) \\
    &\quad - \nabla_W f^{(\ell)}( \nabla_H f^{(\ell+1)}( \ldots \nabla_H f^{(L)}( \mathbf{D}^{(L+1)}_2, \mathbf{H}_2^{(L-1)}, \mathbf{W}_2^{(L)}) \ldots, \mathbf{H}_1^{(\ell)}, \mathbf{W}_1^{(\ell+1)}) , \mathbf{H}_1^{(\ell-1)}, \mathbf{W}_1^{(\ell)}) \|_{\mathrm{F}}^2 \\
    &\quad + \ldots \\
    &\quad + \| \nabla_W f^{(\ell)}( \nabla_H f^{(\ell+1)}( \mathbf{D}_2^{(\ell+2)}, \mathbf{H}_1^{(\ell)}, \mathbf{W}_1^{(\ell+1)}) , \mathbf{H}_1^{(\ell-1)}, \mathbf{W}_1^{(\ell)}) \\
    &\qquad - \nabla_W f^{(\ell)}( \nabla_H f^{(\ell+1)}( \mathbf{D}_2^{(\ell+2)}, \mathbf{H}_2^{(\ell)}, \mathbf{W}_1^{(\ell+1)}) , \mathbf{H}_1^{(\ell-1)}, \mathbf{W}_1^{(\ell)}) \|_{\mathrm{F}}^2 \\
    &\quad + \| \nabla_W f^{(\ell)}( \nabla_H f^{(\ell+1)}( \mathbf{D}_2^{(\ell+2)}, \mathbf{H}_2^{(\ell)}, \mathbf{W}_1^{(\ell+1)}) , \mathbf{H}_1^{(\ell-1)}, \mathbf{W}_1^{(\ell)}) \\
    &\qquad - \nabla_W f^{(\ell)}( \nabla_H f^{(\ell+1)}( \mathbf{D}_2^{(\ell+2)}, \mathbf{H}_2^{(\ell)}, \mathbf{W}_2^{(\ell+1)}) , \mathbf{H}_1^{(\ell-1)}, \mathbf{W}_1^{(\ell)}) \|_{\mathrm{F}}^2 \\
    &\quad + \| \nabla_W f^{(\ell)}( \mathbf{D}_2^{(\ell+1)}, \mathbf{H}_1^{(\ell-1)}, \mathbf{W}_1^{(\ell)}) - \nabla_W f^{(\ell)}( \mathbf{D}_2^{(\ell+1)}, \mathbf{H}_2^{(\ell-1)}, \mathbf{W}_1^{(\ell)}) \|_{\mathrm{F}}^2 \\ 
    &\quad + \| \nabla_W f^{(\ell)}( \mathbf{D}_2^{(\ell+1)}, \mathbf{H}_2^{(\ell-1)}, \mathbf{W}_1^{(\ell)})  - \nabla_W f^{(\ell)}( \mathbf{D}_2^{(\ell+1)}, \mathbf{H}_2^{(\ell-1)}, \mathbf{W}_2^{(\ell)}) \|_{\mathrm{F}}^2 \Big) \\
    \end{aligned}
\end{equation}

By the Lipschitz continuity of $\nabla_W f^{(\ell)}(\cdot)$ and $\nabla_H f^{(\ell)}(\cdot)$
\begin{equation}\label{eq:G_ell_lip_cont}
    \begin{aligned}
     (2L+1)^{-1} \| \mathbf{G}_1^{(\ell)} - \mathbf{G}_2^{(\ell)}\|_{\mathrm{F}}^2 
    &\leq L_{W\ell}^2 L_{H(\ell+1)}^2 \ldots L_{HL}^2 \|\mathbf{D}^{(L+1)}_1 - \mathbf{D}^{(L+1)}_2\|_{\mathrm{F}}^2 \\
    &\quad + L_{W\ell^2} L_{H(\ell+1)}^2 \ldots L_{HL}^2 (\|\mathbf{H}_1^{(L-1)} - \mathbf{H}_2^{(L-1)}\|_{\mathrm{F}}^2 + \|\mathbf{W}_1^{(L)} - \mathbf{W}_2^{(L)}\|_{\mathrm{F}}^2) + \ldots \\
    &\quad + L_{W\ell}^2 L_{H(\ell+1)}^2 (\|\mathbf{H}_1^{(\ell)} - \mathbf{H}_2^{(\ell)}\|_{\mathrm{F}}^2 + \|\mathbf{W}_1^{(\ell+1)} - \mathbf{W}_2^{(\ell+1)}\|_{\mathrm{F}}^2) \\
    &\quad + L_{W\ell}^2 (\|\mathbf{H}_1^{(\ell-1)} - \mathbf{H}_2^{(\ell-1)}\|_{\mathrm{F}}^2 + \|\mathbf{W}_1^{(\ell)} - \mathbf{W}_2^{(\ell)}\|_{\mathrm{F}}^2)  \\
    &\leq U^2_L(\ell, L) L_\text{loss}^2 \|\mathbf{H}_1^{(L)} - \mathbf{H}_2^{(L)}\|_{\mathrm{F}}^2 \\
    &\quad + U^2_L(\ell, L) (\|\mathbf{H}_1^{(L-1)} - \mathbf{H}_2^{(L-1)}\|_{\mathrm{F}}^2 + \|\mathbf{W}_1^{(L)} - \mathbf{W}_2^{(L)}\|_{\mathrm{F}}^2) + \ldots \\
    &\quad + U^2_L(\ell, \ell+1) (\|\mathbf{H}_1^{(\ell)} - \mathbf{H}_2^{(\ell)}\|_{\mathrm{F}}^2 + \|\mathbf{W}_1^{(\ell+1)} - \mathbf{W}_2^{(\ell+1)}\|_{\mathrm{F}}^2) \\
    &\quad + U^2_L(\ell, \ell) (\|\mathbf{H}_1^{(\ell-1)} - \mathbf{H}_2^{(\ell-1)}\|_{\mathrm{F}}^2 + \|\mathbf{W}_1^{(\ell)} - \mathbf{W}_2^{(\ell)}\|_{\mathrm{F}}^2)
    \end{aligned}
\end{equation}
where $U_L(a,b)$ is defined as
\begin{equation}
    U_L(a,b) = \begin{cases}
    L_{Wa} \Big( \prod_{c=a+1}^b L_{Hc} \Big) & \text{ if } b \geq a + 1 \\ 
    L_{Wa}  & \text{ otherwise } 
\end{cases}
\end{equation}

Let define $U_{\max L}$ as
\begin{equation}
   U_{\max L} = \max\Big\{\max_{a,b\in[L]} U_L(a,b), \max_{a,b\in[L]} U_L(a,b) L_\text{loss}\Big\}
\end{equation}
then we can rewrite the above equation as
\begin{equation}
    (2L+1)^{-1} \| \mathbf{G}_1^{(\ell)} - \mathbf{G}_2^{(\ell)}\|_{\mathrm{F}}^2 \leq U_{\max L}^2 \Big( \sum_{j=1}^L \| \mathbf{H}_1^{(j)} - \mathbf{H}_2^{(j)}\|_{\mathrm{F}}^2 \Big) + U_{\max L}^2 \Big( \sum_{j=1}^L \| \mathbf{W}_1^{(j)} - \mathbf{W}_2^{(j)}\|_{\mathrm{F}}^2 \Big)
\end{equation}

Then, let consider the upper bound of $\|\mathbf{H}_1^{(\ell)} - \mathbf{H}_2^{(\ell)}\|_{\mathrm{F}}^2$
\begin{equation}
    \begin{aligned}
    \|\mathbf{H}_1^{(\ell)} - \mathbf{H}_2^{(\ell)}\|_{\mathrm{F}}^2 &= \| f^{(\ell)}(f^{(\ell-1)}(\ldots f^{(1)}(\mathbf{X}, \mathbf{W}_1^{(1)}) \ldots, \mathbf{W}_1^{(\ell-1)}) , \mathbf{W}_1^{(\ell)}) \\
    &\quad - f^{(\ell)}(f^{(\ell-1)}(\ldots f^{(1)}(\mathbf{X}, \mathbf{W}_2^{(1)}) \ldots, \mathbf{W}_2^{(\ell-1)}) , \mathbf{W}_2^{(\ell)}) \|_{\mathrm{F}}^2 \\
    &\leq \| f^{(\ell)}(f^{(\ell-1)}(\ldots f^{(1)}(\mathbf{X}, \mathbf{W}_1^{(1)}) \ldots, \mathbf{W}_1^{(\ell-1)}) , \mathbf{W}_1^{(\ell)}) \\
    &\quad - f^{(\ell)}(f^{(\ell-1)}(\ldots f^{(1)}(\mathbf{X}, \mathbf{W}_2^{(1)}) \ldots, \mathbf{W}_1^{(\ell-1)}) , \mathbf{W}_1^{(\ell)}) \|_{\mathrm{F}}^2 + \ldots \\
    &\quad + \| f^{(\ell)}(f^{(\ell-1)}(\ldots f^{(1)}(\mathbf{X}, \mathbf{W}_2^{(1)}) \ldots, \mathbf{W}_2^{(\ell-1)}) , \mathbf{W}_1^{(\ell)}) \\
    &\quad - f^{(\ell)}(f^{(\ell-1)}(\ldots f^{(1)}(\mathbf{X}, \mathbf{W}_2^{(1)}) \ldots, \mathbf{W}_2^{(\ell-1)}) , \mathbf{W}_1^{(\ell)}) \|_{\mathrm{F}}^2
    \end{aligned}
\end{equation}
By the Lipschitz continuity of $f^{(\ell)}(\cdot, \cdot)$ we have
\begin{equation}
    \begin{aligned}
    \|\mathbf{H}_1^{(\ell)} - \mathbf{H}_2^{(\ell)}\|_{\mathrm{F}}^2 &\leq (C^2_{H\ell} \ldots C^2_{H2} C^2_{W1}) \|\mathbf{W}_1^{(1)} - \mathbf{W}_2^{(1)}\|_{\mathrm{F}}^2 + \ldots + C^2_{W\ell} \|\mathbf{W}_1^{(\ell)} - \mathbf{W}_2^{(\ell)}\|_{\mathrm{F}}^2 \\
    &= U^2_C(1,\ell) \|\mathbf{W}_1^{(1)} - \mathbf{W}_2^{(1)}\|_{\mathrm{F}}^2 + \ldots + U^2_C(\ell, \ell) \|\mathbf{W}_1^{(\ell)} - \mathbf{W}_2^{(\ell)}\|_{\mathrm{F}}^2 \\
    &\leq U_{\max C}^2 \Big( \sum_{j=1}^L \|\mathbf{W}_1^{(j)} - \mathbf{W}_2^{(j)}\|_{\mathrm{F}}^2\Big)
    \end{aligned}
\end{equation}
where $U_C(a,b)$ and $U_{\max C}$ is defined as
\begin{equation}
    U_C(a,b) = \begin{cases}
        C_{Wa} \Big( \prod_{c=a+1}^b C_{Hc} \Big) & \text{ if } b \geq a+1 \\ 
        C_{Wa} & \text{ otherwise } 
\end{cases},~U_{\max C} = \max_{a,b\in[L]} U_C(a,b)
\end{equation}

Plugging it back we have
\begin{equation}
    \| \mathbf{G}_1^{(\ell)} - \mathbf{G}_2^{(\ell)}\|_{\mathrm{F}}^2 \leq (2L+1)(L U_{\max L}^2 U_{\max C}^2 + U_{\max L}^2 ) \Big( \sum_{j=1}^L \| \mathbf{W}_1^{(j)} - \mathbf{W}_2^{(j)}\|_{\mathrm{F}}^2 \Big) 
\end{equation}
Summing both size from $\ell=1$ to $\ell=L$ we have
\begin{equation}
    \begin{aligned}
    \| \nabla \mathcal{L}(\bm{\theta}_1) - \nabla \mathcal{L}(\bm{\theta}_2) \|_{\mathrm{F}}^2 
    &= \sum_{\ell=1}^L \| \mathbf{G}_1^{(\ell)} - \mathbf{G}_2^{(\ell)}\|_{\mathrm{F}}^2 \\
    &\leq L(2L+1)(L U_{\max L}^2 U_{\max C}^2 + U_{\max L}^2 ) \Big( \sum_{j=1}^L \| \mathbf{W}_1^{(j)} - \mathbf{W}_2^{(j)}\|_{\mathrm{F}}^2 \Big) \\
    &\leq L(2L+1)(L U_{\max L}^2 U_{\max C}^2 + U_{\max L}^2 ) \|\bm{\theta}_1 - \bm{\theta}_2\|_{\mathrm{F}}^2
    \end{aligned}
\end{equation}

\end{proof}

\subsection{Remaining steps towards \textcolor{red}{Theorem~?}}
By Lemma~\ref{lemma:smoothness_L_layer} we have
\begin{equation}
    \begin{aligned}
    \mathcal{L}(\bm{\theta}_{t+1}) - \mathcal{L}(\bm{\theta}_t) &\leq  \langle \nabla \mathcal{L}(\bm{\theta}_t), \bm{\theta}_{t+1} - \bm{\theta}_t \rangle + \frac{L_f}{2}\|\bm{\theta}_{t+1} - \bm{\theta}_t\|^2 \\
    &\leq \Big(\frac{L_f}{2}\eta^2-\eta\Big) \| \nabla \mathcal{L}(\bm{\theta}_t) \|^2
    \end{aligned}
\end{equation}
where the smoothness constant is defined in Lemma~\ref{lemma:smoothness_L_layer}.

Summing over $t=1$ to $t=T$ we have
\begin{equation}
    \begin{aligned}
    \eta \Big(1-\frac{L_f}{2}\eta\Big) \sum_{t=1}^T \| \nabla \mathcal{L}(\bm{\theta}_t) \|^2 &\leq \mathcal{L}(\bm{\theta}_1) - \mathcal{L}(\bm{\theta}_{T+1}) \\
    &\leq \mathcal{L}(\bm{\theta}_1) - \mathcal{L}(\bm{\theta}^\star)
    \end{aligned}
\end{equation}

Let $\eta = 1/L_f$ and rearranging it, we have
\begin{equation}
    \frac{1}{T}\sum_{t=1}^T \| \nabla \mathcal{L}(\bm{\theta}_t) \|^2 \leq \frac{2L_f(\mathcal{L}(\bm{\theta}_1) - \mathcal{L}(\bm{\theta}^\star))}{T}
\end{equation}
