# Supplementary material for: On the Importance of Sampling in Training GCNs: Tighter Analysis and Variance Reduction
Source: arXiv:2103.02696 source file (2021-11-01)
Supplement: Supplementary file 10 [file experiment_details.tex]

% \section{Experiment configurations}\label{section:exp-config}

% \noindent\textbf{Hardware specification and environment.}~
% We run our experiments on a single machine with Intel i9-10850K, NVIDIA GTX3090 GPU (24GB memory) and, 32GB RAM memory. 
% The code is written in Python 3.7 and we use PyTorch 1.4 on CUDA 10.1 to train the model on GPU. 
% During each epoch, we randomly construct 10 mini-batches in parallel. 

% \noindent\textbf{Implementation details.}~
% To demonstrate the effectiveness of doubly variance reduction, we modified the PyTorch implementation of {GCN}~\cite{semigcn}\footnote{\url{https://github.com/tkipf/pygcn}} to add \texttt{LADIES}~\cite{ladies}, \texttt{FastGCN}~\cite{fastgcn}, \texttt{GraphSAGE}~\cite{graphsage}, \texttt{GraphSAINT}~\cite{graphsaint}, \texttt{VRGCN}~\cite{control_variacne_gcn}, and \texttt{Exact} sampling mechanism. 
% Then, we implement \texttt{SGCN+} and \texttt{SGCN++} on the top of each sampling method to illustrate how zeroth-order variance reduction and doubly variance reduction help for GCN training. 
% The source code for our experiments is available on \href{https://anonymous.4open.science/r/68b416be-b4c8-432c-b2c8-604fa339f81f/}{https://anonymous.4open.science/r/68b416be-b4c8-432c-b2c8-604fa339f81f/}.

% By default, we train $2$-layers GCNs with hidden state dimension of $256$, element-wise ELU as the activation function and symmetric normalized Laplacian matrix $\mathbf{L} = \mathbf{D}^{-1/2} \mathbf{A} \mathbf{D}^{-1/2}$. 
% We use \emph{mean-aggregation} for single-class classification task and \emph{concatenate-aggregation} for multi-class classification.
% The default mini-batch batch size and sampled node size are summarized in Table~\ref{table:train_config}.
% We update the model using Adam optimizer with a learning rate of $0.01$. 
% For \texttt{SGCN++}, historical node embeddings are first calculated on GPUs and transfer to CPU memory using PyTorch command \texttt{Tensor.to(device)}. 
% Therefore, no extra GPU memory is required when training with \texttt{SGCN++}. 
% To balance the staleness of snapshot model and the computational efficiency, as default we choose snapshot gap $K=10$ and early stop inner-loop if the Euclidean distance between current step gradient to snapshot gradient is larger than $0.002$ times the norm of snapshot gradient.

% \input{supplementary/experiment_configs}

% During training, for each epoch we construct $10$ mini-batches in parallel using Python package \texttt{multiprocessing} and perform training on the sampled $10$ mini-batches. 
% To achieves a fair comparison of different sampling strategies in terms of sampling complexity, we implement all sampling algorithms using \texttt{numpy.random} and \texttt{scipy.sparse} package. 

% We have to emphasize that, in order to better observe the impact of sampling on convergence, we have not use any augmentation methods (e.g., ``layer normalization'', ``skip-connection'', and ``attention''), which have been proven to impact the GCN performance in~\cite{cai2020graphnorm,dwivedi2020benchmarkgnns}.
% Notice that we are not criticizing the usage of these augmentations. 
% Instead, we use the most primitive network structure to better explore the impact of sampling and variance reduction on convergence.

% \noindent\textbf{Comparison of SGD and Adam.}
% It is worth noting that Adam optimizer is used as the default optimizer during training. We choose Adam optimizer over SGD optimizer for the following reasons: 
% \begin{itemize}
%     \item [(a)] Baseline methods training with SGD cannot converge when using a constant learning rate due to the bias and variance in stochastic gradient (Adam has some implicit variance reduction effect, which can alleviate the issue). 
%     The empirical result of SGD trained baseline models has a huge performance gap to the one trained with Adam, which makes the comparison meaningless. 
%     For example in Figure~\ref{fig:sgd_vs_adam_ppi}, we compare Adam and SGD optimizer on PPI dataset. For Adam optimizer we use PyTorch's default learning rate $0.01$, and for SGD optimizer we choose learning rate as $0.1$, which is selected as the most stable learning rate from range $[0.01, 1]$ for this dataset. Although the SGD is using a learning rate $10$ times larger than Adam, it requires $100$ times more iterations than Adam to reach the early stop point (valid loss do not decrease for $200$ iterations), and suffers a giant performance gap when comparing to Adam optimizer. 
%     \item [(b)] Most public implementation of GCNs, including all implementations in PyTorch Geometric and DGL packages, use Adam optimizer instead of SGD optimizer.
%     \item [(c)] In this paper, we mainly focus on how to estimate a stabilized stochastic gradient, instead of how to take the existing gradient for weight update. 
%     We employ Adam optimizer for all algorithms during experiment, which lead to a fair comparison.
% \end{itemize}

% \begin{figure}
%     \centering
%     \includegraphics[width=0.9\textwidth]{figures/sgd_vs_adam_ppi.pdf}
%     \caption{Comparison of doubly variance reduction and vanilla sampling-based GCN training on PPI dataset with SGD (learning rate $0.1$) and Adam optimizer (learning rate $0.01$). All other configurations are as default.}
%     \label{fig:sgd_vs_adam_ppi}
% \end{figure}

% \noindent\textbf{Dataset statistics.}~
% We summarize the dataset statistics in Table~\ref{table:datasets}.

% \begin{table}[h]
% \vspace{0mm}
% \caption{Summary of dataset statistics. 
% \textbf{m} stands for \textbf{m}ulti-class classification, and \textbf{s} stands for \textbf{s}ingle-class.
% }
% \label{table:datasets}
% \centering
% % \scalebox{1.0}{ %arxiv
% \begin{tabular}{rcccccc}
% \toprule
% \textbf{Dataset}   & \textbf{Nodes} & \textbf{Edges} & \textbf{Degree} & \textbf{Feature} & \textbf{Classes} & \textbf{Train/Val/Test} \\ \midrule
% % \textbf{Pubmed}    & 19,717         & 44,338         & 3               & 500              & 3(\textbf{s})          & 92\%/~3\%/~5\%          \\ \hline
% \textbf{PPI}       & $14,755$         & $225,270$        & $15$              & $50$               & $121$(\textbf{m})          & $66\%/12\%/22\%$          \\ 
% \textbf{PPI-Large} & $56,944$         & $818,716$        & $14$              & $50$               & $121$(\textbf{m})          & $79\%/11\%/10\%$          \\ 
% \textbf{Flickr}    & $89,250$         & $899,756$        & $10$              & $500$              & $7$ (\textbf{s})               & $50\%/25\%/25\%$          \\ 
% \textbf{Reddit}    & $232,965$        & $11,606,919$     & $50$              & $602$              & $41$(\textbf{s})               & $66\%/10\%/24\%$          \\ 
% \textbf{Yelp}      & $716,847$        & $6,977,410$      & $10$              & $300$              & $100$(\textbf{m})          & $75\%/10\%/15\% $         \\ 
% \bottomrule
% % \textbf{Amazon}    & 1,598,960      & 132,169,734    & 83              & 200              & 107(\textbf{m})          & 85\%/5\%/10\%          \\ \hline
% \end{tabular}
% % }
% \vskip -0.1in
% \end{table}
